# Supplementary material for: Optical phonons for Peierls chains with long-range Coulomb interactions
Source: arXiv:1611.04335 source file (2016-11-14)
Supplement: Supplementary file 1 [file timar-barcza-supp.pdf]

# Supplemental Material for
# Optical phonons for Peierls chains with long-range Coulomb interactions

Máté Timár[1,2], Gergely Barcza[1], Florian Gebhard[3,*] and Örs Legeza[1†]
[1] *Strongly Correlated Systems Lendület Research Group, Institute for Solid State Physics and Optics, MTA Wigner Research Centre for Physics, P.O. Box 49, H-1525 Budapest, Hungary*
[2] *Department of Physics of Complex Systems, Eötvös University, H-1117 Budapest, Hungary and*
[3] *Fachbereich Physik, Philipps-Universität Marburg, D-35032 Marburg, Germany*
(Dated: Version of September 15, 2016)

For comparison with our results in the main text, we derive the phonon dispersion in a straight Peierls chain. We include the derivation of the Hellmann-Feynman theorem to first and second order and the derivation of energy gradients.

## I. PHONON DISPERSION IN A PEIERLS CHAIN

### A. Model and ground-state properties

#### 1. Peierls Hamiltonian

We consider electrons on a ring with $2L$ sites at positions $x_l$; periodic boundary conditions apply. The system is half filled, i.e., the number of electrons equals the number of sites, $N = 2L$; the system is paramagnetic, $N_\uparrow = N_\downarrow = L$.

The electrons move between neighboring sites. The undistorted lattice spacing is $r_0 = 1.4\,\text{Å}$. The lattice can slightly dimerize due to the Peierls effect,

$$x_l = lr_0 + u_l \quad , \quad |u_l| \ll r_0 \; . \tag{1}$$

The electron transfer amplitudes between sites $l$ and $l+1$ are modified accordingly,

$$t_l(\{u_n\}) = t_0(1+\delta_l) = t_0 - \alpha_x(u_{l+1} - u_l) \; , \tag{2}$$

where $t_0 = 2.5\,\text{eV}$ is the electron transfer amplitude between undistorted neighboring lattice sites and $\alpha_x = 4.1\,\text{eV/Å}$ is the Peierls-coupling constant used in Ref. [1]. For small, static lattice distortions, the energy of the system increases by the potential energy

$$V_{\text{latt}}(\{u_n\}) = \frac{K_x}{2}\sum_{l=1}^{2L}(u_{l+1}-u_l)^2 \tag{3}$$

with the spring constant $K_x = 21\,\text{eV/Å}^2$.[1] When we treat the lattice distortions adiabatically and ignore the Coulomb interaction between the electrons, we end up with the Peierls model,

$$\begin{aligned}\hat{H} = -\sum_\sigma\sum_{l=1}^{2L} t_l(\{u_n\})\left(\hat{c}^\dagger_{l+1,\sigma}\hat{c}_{l,\sigma} + \hat{c}^\dagger_{l,\sigma}\hat{c}_{l+1,\sigma}\right)\\ +V_{\text{latt}}(\{u_n\})\end{aligned} \tag{4}$$

in standard notation for the Fermi operators $\hat{c}_{l,\sigma}$ for electrons with spin $\sigma = \uparrow, \downarrow$, and with $t_l(\{u_n\})$ from eq. (2) and $V_{\text{latt}}(\{u_n\})$ from eq. (3).

#### 2. Ground state at half band-filling

The half-filled ground state is readily found because the Peierls wave number is commensurate with the Fermi wave number of the undistorted lattice,[2]

$$\begin{aligned} u_l^{(0)} &= (-1)^l\frac{u}{2} \; ,\\ x_{l+1} - x_l &= r_0 + u(-1)^{l+1} \; ,\\ t_l &= t_0(1+(-1)^l\delta) \; ,\\ \delta &= \frac{\alpha_x u}{t_0} \; . \end{aligned} \tag{5}$$

We must diagonalize the kinetic energy

$$\begin{aligned}\hat{T}(\delta) = -t_d\sum_{l=1,\sigma}^{L}\hat{c}^\dagger_{2l,\sigma}\hat{c}_{2l+1,\sigma} + \hat{c}^\dagger_{2l+1,\sigma}\hat{c}_{2l,\sigma}\\ -t_s\sum_{l=1,\sigma}^{L}\hat{c}^\dagger_{2l-1,\sigma}\hat{c}_{2l,\sigma} + \hat{c}^\dagger_{2l-1,\sigma}\hat{c}_{2l,\sigma} \; ,\end{aligned} \tag{6}$$

where $t_d = t_0(1+\delta)$ and $t_s = t_0(1-\delta)$ are the electron transfer amplitudes for short ('double') and long ('single') bonds. The diagonalization is readily achieved in momentum space.[1,3] For periodic boundary conditions, we introduce the Fourier transformed electron operators

$$\begin{aligned}\hat{c}^\dagger_{k,\sigma} &= \sqrt{\frac{1}{2L}}\sum_{l=1}^{2L}e^{\mathrm{i}kl}\hat{c}^\dagger_{l,\sigma} \; ,\\ \hat{c}^\dagger_{l,\sigma} &= \sqrt{\frac{1}{2L}}\sum_{|k|\leq\pi/2}e^{-\mathrm{i}kl}\left(\hat{c}^\dagger_{k,\sigma} + (-1)^l\hat{c}^\dagger_{k+\pi,\sigma}\right)\end{aligned} \tag{7}$$

for the momenta $k = 2\pi m/(2L)$, $m = -L/2+1, \ldots, L/2$ from the reduced Brillouin zone. We may thus write

$$\begin{aligned}\hat{T}(\delta) = \sum_{|k|\leq\pi/2,\sigma}\epsilon(k)\left(\hat{c}^\dagger_{k,\sigma}\hat{c}_{k,\sigma} - \hat{c}^\dagger_{k+\pi,\sigma}\hat{c}_{k+\pi,\sigma}\right)\\ -\mathrm{i}\Delta(k)\left(\hat{c}^\dagger_{k+\pi,\sigma}\hat{c}_{k,\sigma} - \hat{c}^\dagger_{k,\sigma}\hat{c}_{k+\pi,\sigma}\right)\end{aligned} \tag{8}$$

with the dispersion relation $\epsilon(k)$ and hybridization function $\Delta(k)$ defined as

$$\begin{aligned}\epsilon(k) &= (t_d + t_s)\cos(k) = -2t_0\cos(k) \; ,\\ \Delta(k) &= (t_d - t_s)\sin(k) = 2t_0\delta\sin(k) \; .\end{aligned} \tag{9}$$

The Hamiltonian is diagonalized in $k$-space by introducing the Fermion quasi-particle operators for the Peierls bands $\hat{a}^{+}_{k,\sigma,\pm}$. They are related to the original electron operators by

$$\begin{aligned}\hat{a}_{k,\sigma,-} &= \alpha_k \hat{c}_{k,\sigma} + \mathrm{i}\beta_k \hat{c}_{k+\pi,\sigma} \ , \\ \hat{a}_{k,\sigma,+} &= \beta_k \hat{c}_{k,\sigma} - \mathrm{i}\alpha_k \hat{c}_{k+\pi,\sigma}\end{aligned} \tag{10}$$

for $|k| \leq \pi/2$. The inverse transformation reads

$$\begin{aligned}\hat{c}_{k,\sigma} &= \alpha_k \hat{a}_{k,\sigma,-} + \beta_k \hat{a}_{k,\sigma,+} \ , \\ \hat{c}_{k+\pi,\sigma} &= -\mathrm{i}\beta_k \hat{a}_{k,\sigma,-} + \mathrm{i}\alpha_k \hat{a}_{k,\sigma,+} \ ,\end{aligned} \tag{11}$$

where $\alpha_k^2 + \beta_k^2 = 1$ has to be fulfilled for a canonical transformation.

We note the helpful relations

$$\begin{aligned}\hat{c}^{\dagger}_{k,\sigma}\hat{c}_{k,\sigma} - \hat{c}^{\dagger}_{k+\pi,\sigma}\hat{c}_{k+\pi,\sigma} &= \left(\alpha_k^2 - \beta_k^2\right)\left(\hat{n}_{k,\sigma,-} - \hat{n}_{k,\sigma,+}\right) \\ &\quad +2\alpha_k\beta_k\left(\hat{P}_{k,\sigma} + \hat{P}^{\dagger}_{k,\sigma}\right) \\ \hat{c}^{\dagger}_{k,\sigma}\hat{c}_{k,\sigma} + \hat{c}^{\dagger}_{k+\pi,\sigma}\hat{c}_{k+\pi,\sigma} &= \hat{n}_{k,\sigma,-} + \hat{n}_{k,\sigma,+} \\ \hat{c}^{\dagger}_{k,\sigma}\hat{c}_{k+\pi,\sigma} - \hat{c}^{\dagger}_{k+\pi,\sigma}\hat{c}_{k,\sigma} &= \mathrm{i}\left(\alpha_k^2 - \beta_k^2\right)\left(\hat{P}^{\dagger}_{k,\sigma} + \hat{P}_{k,\sigma}\right) \\ &\quad +\mathrm{i}2\alpha_k\beta_k\left(\hat{n}_{k,\sigma,+} - \hat{n}_{k,\sigma,-}\right) \\ \hat{c}^{\dagger}_{k,\sigma}\hat{c}_{k+\pi,\sigma} + \hat{c}^{\dagger}_{k+\pi,\sigma}\hat{c}_{k,\sigma} &= -\mathrm{i}\left(\hat{P}^{\dagger}_{k,\sigma} - \hat{P}_{k,\sigma}\right) \ ,\end{aligned} \tag{12}$$

where $\hat{n}_{k,\sigma,\pm} = \hat{a}^{\dagger}_{k,\sigma,\pm}\hat{a}_{k,\sigma,\pm}$, $\hat{P}_{k,\sigma} = \hat{a}^{\dagger}_{k,\sigma,-}\hat{a}_{k,\sigma,+}$, and $\hat{P}^{\dagger}_{k,\sigma} = \hat{a}^{\dagger}_{k,\sigma,+}\hat{a}_{k,\sigma,-}$. They allow us to write the Hamiltonian in momentum space, eq. (8), as

$$\begin{aligned}\hat{T}(\delta) &= \sum_{|k|\leq\pi/2,\sigma}\left(\hat{n}_{k,\sigma,+} - \hat{n}_{k,\sigma,-}\right) \\ &\qquad \times\left[-\epsilon(k)(\alpha_k^2 - \beta_k^2) - \Delta(k)2\alpha_k\beta_k\right] \\ &\quad + \sum_{|k|\leq\pi/2,\sigma}\left(\hat{P}^{\dagger}_{k,\sigma} + \hat{P}_{k,\sigma}\right) \\ &\qquad \times\left[\epsilon(k)2\alpha_k\beta_k - \Delta(k)(\alpha_k^2 - \beta_k^2)\right] .\end{aligned} \tag{13}$$

We demand that the mixing terms vanish. This gives the following relation between $\alpha_k = \cos\phi_k$ and $\beta_k = \sin\phi_k$

$$\tan(2\phi_k) = \frac{\Delta(k)}{\epsilon(k)} \ . \tag{14}$$

The mixing amplitudes become

$$\begin{aligned}2\alpha_k\beta_k &= -\frac{\Delta(k)}{E(k)} \ , \\ \alpha_k^2 - \beta_k^2 &= -\frac{\epsilon(k)}{E(k)} \ , \\ \alpha_k &= \sqrt{\frac{1}{2}\left(1 - \frac{\epsilon(k)}{E(k)}\right)} \ , \\ \beta_k &= -\sqrt{\frac{1}{2}\left(1 + \frac{\epsilon(k)}{E(k)}\right)}\mathrm{sgn}\left(\Delta(k)\right) \ ,\end{aligned} \tag{15}$$

where $\mathrm{sgn}(x)$ is the sign function and $\alpha_{k+\pi} = -\mathrm{i}\beta_k$, $\beta_{k+\pi} = \mathrm{i}\alpha_k$. The kinetic energy is diagonal in the new operators,

$$\hat{T}(\delta) = \sum_{|k|\leq\pi/2,\sigma} E(k)\left(\hat{n}_{k,\sigma,+} - \hat{n}_{k,\sigma,-}\right) \ . \tag{16}$$

Here, $\pm E(k)$ is the dispersion relation for the upper $(+)$ and lower $(-)$ Peierls band,

$$E(k) = \sqrt{\epsilon(k)^2 + \Delta(k)^2} \ . \tag{17}$$

The ground state is the Peierls insulator,

$$|\Psi_0(u)\rangle = \prod_{\sigma}\prod_{k,|k|\leq\pi/2}\hat{a}^{\dagger}_{k,\sigma,-}|\mathrm{vac}\rangle \ . \tag{18}$$

The gap for single-particle excitations is obtained from $E_{\mathrm{gap}}(u) = 2\Delta(\pi/2) = 4t_0\delta = 4\alpha_x u$.

#### 3. *Ground-state lattice distortion*

The remaining task is to determine the lattice distortion in the ground state. Including the lattice energy, the ground-state energy density in the thermodynamic limit reads

$$e_0(u) = \lim_{L\to\infty}\left(\frac{E_0(u)}{2L}\right) = \frac{K_x}{2}u^2 - 2\int_{-\pi/2}^{\pi/2}\frac{\mathrm{d}k}{2\pi}E(k) \ . \tag{19}$$

It has to be minimized with respect to $u$ which leads to the implicit equation ($u_0 \neq 0$)

$$\frac{K_x t_0}{4\alpha_x^2} = \int_{-\pi/2}^{\pi/2}\frac{\mathrm{d}k}{2\pi}\frac{\sin^2(k)}{\sqrt{\cos^2(k) + \delta_0^2\sin^2(k)}} \ . \tag{20}$$

Eq. (20) fixes the value for $\delta_0 = \alpha_x u_0/t_0$ as a function of $K_x t_0/(4\alpha_x^2)$. For $t_0 = 2.5\,\mathrm{eV}$, $\alpha_x = 4.1\,\mathrm{eV/Å}$, and $K_x = 21\,\mathrm{eV/Å^2}$, we find using MATHEMATICA[4] $\delta_0 = 0.130$ so that $u_0 = 0.079\,\mathrm{Å}$. The single-particle gap is $E_{\mathrm{gap}}(u_0) = 1.3\,\mathrm{eV}$.

### B. Phonons

#### 1. *Perturbation Hamiltonian*

We distort the lattice around the Peierls-deformed configuration,

$$u_l = u_l^{(0)} + \eta_l \quad , \quad |\eta_l| \ll u_0 \ . \tag{21}$$

Recall that $u_l^{(0)} = (-1)^l u_0/2$. Then, the lattice energy becomes

$$
\begin{aligned}
V_{\rm latt} &= (2L)\frac{K_x}{2}u_0^2 + V_{\rm latt}^{(1)} + V_{\rm latt}^{(2)} \; , \\
V_{\rm latt}^{(1)} &= 2K_x u_0 \sum_{l=1}^{2L}(-1)^l \eta_l \; , \\
V_{\rm latt}^{(2)} &= \frac{K_x}{2}\sum_{l=1}^{2L}(\eta_{l+1}-\eta_l)^2 \; . \qquad (22)
\end{aligned}
$$

We transfer into Fourier space,

$$
\widetilde{\eta}_q = \sqrt{\frac{1}{2L}}\sum_l e^{{\rm i}ql}\eta_l \quad , \quad \eta_l = \sqrt{\frac{1}{2L}}\sum_q e^{-{\rm i}ql}\widetilde{\eta}_q \; , \qquad (23)
$$

for $q = (2\pi/2L)m_q$, $m_q = -L+1,\ldots,L$, and find

$$
\begin{aligned}
V_{\rm latt}^{(1)} &= 2K_x u_0\sqrt{L}\widetilde{\eta}_\pi \; , \\
V_{\rm latt}^{(2)} &= \frac{K_x}{2}\sum_q 4[\sin(q/2)]^2|\widetilde{\eta}_q|^2 \; , \qquad (24)
\end{aligned}
$$

where we used the fact that $\eta_l$ is real so that $\widetilde{\eta}_{-q} = \widetilde{\eta}_q^*$.

Since we have

$$
t_l = t_0(1+(-1)^l\delta) - \alpha_x(\eta_{l+1}-\eta_l) \; , \qquad (25)
$$

we identify the perturbation Hamiltonian as

$$
\hat{H}_\perp = \alpha_x\sum_{l,\sigma}(\eta_{l+1}-\eta_l)\left(\hat{c}_{l+1,\sigma}^\dagger\hat{c}_{l,\sigma} + \hat{c}_{l,\sigma}^\dagger\hat{c}_{l+1,\sigma}\right) \; . \qquad (26)
$$

In Fourier space it reads

$$
\hat{H}_\perp = \alpha_x\sqrt{\frac{1}{L}}{\sum_{k,p,\sigma}}' \mu(k,p)\hat{c}_{k,\sigma}^\dagger\hat{c}_{p,\sigma} \; , \qquad (27)
$$

where the momenta are from the reduced Brillouin zone, $|k|,|p| \leq \pi/2$, as indicated by the prime on the sum. Moreover,

$$
\mu(k,p) = \widetilde{\eta}_{p-k}f_{k,p} \quad , \quad f_{k,p} = 2{\rm i}(\sin(k)-\sin(p)) \; . \qquad (28)
$$

In terms of the Peierls operators, the perturbation reads

$$
\begin{aligned}
\hat{H}_\perp = {} & \alpha_x\sqrt{\frac{1}{L}}{\sum_{k,p,\sigma}}'\mu(k,p) \\
& \Big[(\alpha_k\hat{a}_{k,\sigma,-}^\dagger + \beta_k\hat{a}_{k,\sigma,+}^\dagger)(\alpha_p\hat{a}_{p,\sigma,-} + \beta_p\hat{a}_{p,\sigma,+}) \\
& -({\rm i}\beta_k\hat{a}_{k,\sigma,-}^\dagger - {\rm i}\alpha_k\hat{a}_{k,\sigma,+}^\dagger)(-{\rm i}\beta_p\hat{a}_{p,\sigma,-} + {\rm i}\alpha_p\hat{a}_{p,\sigma,+})\Big] \\
& +\alpha_x\sqrt{\frac{1}{L}}{\sum_{k,p,\sigma}}'\mu(k+\pi,p) \\
& \Big[({\rm i}\beta_k\hat{a}_{k,\sigma,-}^\dagger - {\rm i}\alpha_k\hat{a}_{k,\sigma,+}^\dagger)(\alpha_p\hat{a}_{p,\sigma,-} + \beta_p\hat{a}_{p,\sigma,+}) \\
& -(\alpha_k\hat{a}_{k,\sigma,-}^\dagger + \beta_k\hat{a}_{k,\sigma,+}^\dagger)(-{\rm i}\beta_p\hat{a}_{p,\sigma,-} + {\rm i}\alpha_p\hat{a}_{p,\sigma,+})\Big] \; . \qquad (29)
\end{aligned}
$$

### 2. First-order correction

To first order in perturbation theory we have

$$
\langle\Psi_0(u_0)|\hat{H}_\perp|\Psi_0(u_0)\rangle = \alpha_x\sqrt{\frac{1}{L}}{\sum_{k,\sigma}}'\mu(k+\pi,k)2{\rm i}\alpha_k\beta_k \; , \qquad (30)
$$

where we used that $\mu(k,k) = 0$ so that the first term in (29) gives a vanishing contribution. Using eqs. (15), (20), and (28), we find

$$
\begin{aligned}
\langle\Psi_0(u_0)|\hat{H}_\perp|\Psi_0(u_0)\rangle &= -4\alpha_x\sqrt{L}\widetilde{\eta}_\pi \\
& \int_{-\pi/2}^{\pi/2}\frac{{\rm d}k}{\pi}\frac{\delta_0\sin^2(k)}{\sqrt{\cos^2(k)+\delta_0^2\sin^2(k)}} \\
&= -2u_0K_x\sqrt{L}\widetilde{\eta}_\pi \\
&= -V_{\rm latt}^{(1)} \; . \qquad (31)
\end{aligned}
$$

Therefore, the lattice energy $V_{\rm latt}^{(1)}$ cancels the electronic contribution from $\hat{H}_\perp$ and there is no energy correction to first order, as it should.

### 3. Second-order correction

Since $\hat{H}_\perp$ is bi-linear in the Fermi operators, all excited states $|m\rangle$ that can be reached from $|\Psi_0(u_0)\rangle$ contain a hole in the lower Peierls band at momentum $p$ and a particle in the upper Peierls band at momentum $k$, i.e., we may write $|m\rangle \equiv |k;p\rangle = \hat{a}_{k,\sigma,+}^+\hat{a}_{p,\sigma,-}|\Psi_0(u_0)\rangle$. The correction to the ground-state energy to second order becomes

$$
E_0^{(2)} = -2\frac{\alpha_x^2}{2L}{\sum_{k,p}}'\frac{\left|\langle k;p|\hat{H}_\perp|\Psi_0(u_0)\rangle\right|^2}{E(k)+E(p)} \; , \qquad (32)
$$

where we summed over the spin index. Using eq. (29) we find

$$
\begin{aligned}
E_0^{(2)} &= -2\frac{\alpha_x^2}{L}{\sum_{k,p}}'\frac{|A_{k,p}|^2}{E(k)+E(p)} \\
A_{k,p} &= \widetilde{\eta}_{p-k}f_{k,p}(\alpha_p\beta_k + \beta_p\alpha_k) \\
& \quad +\widetilde{\eta}_{p-k+\pi}f_{k+\pi,p}(-{\rm i})(\alpha_k\alpha_p - \beta_k\beta_p) \; . \qquad (33)
\end{aligned}
$$

In the following we set $p = k+q$ and concentrate on $0 \leq q \leq \pi/2$ because the system is inversion symmetric. In the thermodynamic limit we obtain

$$
\begin{aligned}
E_0^{(2)} &= \sum_q E_0^{(2)}(q) \; , \\
E_0^{(2)}(q) &= -8\alpha_x^2\int_{-\pi/2}^{\pi/2-q}\frac{{\rm d}k}{2\pi}\frac{|B_{k,k+q}|^2}{E(k)+E(k+q)} \\
& \quad -8\alpha_x^2\int_{\pi/2-q}^{\pi/2}\frac{{\rm d}k}{2\pi}\frac{|C_{k,k+q}|^2}{E(k)+E(k+q)} \; , \qquad (34)
\end{aligned}
$$

where

$$B_{k,k+q} = \mathrm{i}\widetilde{\eta}_q \left[\sin(k) - \sin(k+q)\right] \left(\alpha_{k+q}\beta_k + \beta_{k+q}\alpha_k\right) \\ -\widetilde{\eta}_{q+\pi} \left[\sin(k) + \sin(k+q)\right] \left(\alpha_k\alpha_{k+q} - \beta_k\beta_{k+q}\right) \tag{35}$$

and

$$C_{k,k+q} = \widetilde{\eta}_q \left[\sin(k) - \sin(k+q)\right] \\ \times \left(\alpha_k\alpha_{k+q-\pi} - \beta_k\beta_{k+q-\pi}\right) \\ -\mathrm{i}\widetilde{\eta}_{q+\pi} \left[\sin(k) + \sin(k+q)\right] \\ \times \left(\alpha_{k+q-\pi}\beta_k + \beta_{k+q-\pi}\alpha_k\right) \ . \tag{36}$$

We collect the four contributions from the distortion in momentum space and write

$$E_0^{(2)}(q) = \widetilde{\eta}_q^*\widetilde{\eta}_q D_{11}(q) + \widetilde{\eta}_q^*\widetilde{\eta}_{q+\pi} D_{12}(q) \\ +\widetilde{\eta}_{q+\pi}^*\widetilde{\eta}_q D_{21}(q) + \widetilde{\eta}_{q+\pi}^*\widetilde{\eta}_{q+\pi} D_{22}(q) \ . \tag{37}$$

The matrix entries $D_{mn}(q)$ read explicitly

$$D_{11}(q) = -8\alpha_x^2 \int_{-\pi/2}^{\pi/2-q} \frac{\mathrm{d}k}{2\pi} \frac{\left[\sin(k) - \sin(k+q)\right]^2}{E(k) + E(k+q)} \\ \times \left(\alpha_{k+q}\beta_k + \beta_{k+q}\alpha_k\right)^2 \\ -8\alpha_x^2 \int_{-\pi/2-q}^{\pi/2} \frac{\mathrm{d}k}{2\pi} \frac{\left[\sin(k) - \sin(k+q)\right]^2}{E(k) + E(k+q)} \\ \times \left(\alpha_{k+q-\pi}\alpha_k - \beta_{k+q-\pi}\beta_k\right)^2 \ , \tag{38}$$

$$D_{12}(q) = -8\mathrm{i}\alpha_x^2 \int_{-\pi/2}^{\pi/2-q} \frac{\mathrm{d}k}{2\pi} \frac{\left[\sin^2(k) - \sin^2(k+q)\right]}{E(k) + E(k+q)} \\ \times \left(\alpha_{k+q}\beta_k + \beta_{k+q}\alpha_k\right) \\ \times \left(\alpha_k\alpha_{k+q} - \beta_k\beta_{k+q}\right) \\ +8\mathrm{i}\alpha_x^2 \int_{\pi/2-q}^{\pi/2} \frac{\mathrm{d}k}{2\pi} \frac{\left[\sin^2(k) - \sin^2(k+q)\right]}{E(k) + E(k+q)} \\ \times \left(\alpha_{k+q-\pi}\alpha_k - \beta_{k+q-\pi}\beta_k\right) \\ \times \left(\alpha_k\beta_{k+q-\pi} + \beta_k\alpha_{k+q-\pi}\right) \\ = \left[D_{21}(q)\right]^* \ , \tag{39}$$

$$D_{22}(q) = -8\alpha_x^2 \int_{-\pi/2}^{\pi/2-q} \frac{\mathrm{d}k}{2\pi} \frac{\left[\sin(k) + \sin(k+q)\right]^2}{E(k) + E(k+q)} \\ \times \left(\alpha_k\alpha_{k+q} - \beta_k\beta_{k+q}\right)^2 \\ -8\alpha_x^2 \int_{\pi/2-q}^{\pi/2} \frac{\mathrm{d}k}{2\pi} \frac{\left[\sin(k) + \sin(k+q)\right]^2}{E(k) + E(k+q)} \\ \times \left(\alpha_k\beta_{k+q-\pi} + \beta_k\alpha_{k+q-\pi}\right)^2 \ . \tag{40}$$

The classical Hamilton function for the motion of atoms with mass $M$ in a Peierls chain reads in momentum space

$$\mathcal{H} = \frac{M}{2}\sum_q \left(\dot{\widetilde{\eta}}_q^*\dot{\widetilde{\eta}}_q + \dot{\widetilde{\eta}}_{q+\pi}^*\dot{\widetilde{\eta}}_{q+\pi}\right) \\ +\sum_q \left(E_0^{(2)}(q) + V_{\mathrm{latt}}^{(2)}(q)\right) \ , \tag{41}$$

with $E_0^{(2)}(q)$ from eq. (37). The lattice energy (24) is given by

$$V_{\mathrm{latt}}^{(2)}(q) = \widetilde{\eta}_q^*\widetilde{\eta}_q V_{11}(q) + \widetilde{\eta}_{q+\pi}^*\widetilde{\eta}_{q+\pi} V_{22}(q) \tag{42}$$

with

$$V_{11}(q) = 2K_x\sin^2(q/2) \quad , \quad V_{22}(q) = 2K_x\cos^2(q/2) \ . \tag{43}$$

In order to find the phonon frequencies we have to consider the matrix $\underline{\underline{\Omega}}(q)$ with the entries

$$\Omega_{11}(q) = M\omega(q)^2/2 - D_{11}(q) - V_{11}(q) \\ \Omega_{12}(q) = -D_{12}(q) \\ \Omega_{21}(q) = -D_{21}(q) = -\left[D_{12}(q)\right]^* \\ \Omega_{22}(q) = M\omega(q)^2/2 - D_{22}(q) - V_{22}(q) \ . \tag{44}$$

The secular equation $\det\left(\underline{\underline{\Omega}}(q)\right) = 0$ for each $-\pi/2 \leq q \leq \pi/2$ gives the dispersion relations

$$\frac{\left[\omega^{\mathrm{ac,opt}}(q)\right]^2}{4K_x/M} = \frac{1}{2}\left[1 + \frac{D_{11}(q) + D_{22}(q)}{2K_x} \pm \sqrt{D(q)}\right] , \\ D(q) = \left(1 + \frac{D_{11}(q) + D_{22}(q)}{2K_x}\right)^2 + \left|\frac{D_{12}(q)}{K_x}\right|^2 \\ -4\left(\frac{D_{11}(q)}{2K_x} + \sin^2(q/2)\right) \\ \times\left(\frac{D_{22}(q)}{2K_x} + \cos^2(q/2)\right) \tag{45}$$

for the acoustic ($-$) and optical ($+$) phonon branch. The result agrees with expressions derived earlier by other authors.[5–7] The phonon dispersions are shown in Fig. 1. We discuss their general features together with the analysis of interesting limiting cases.

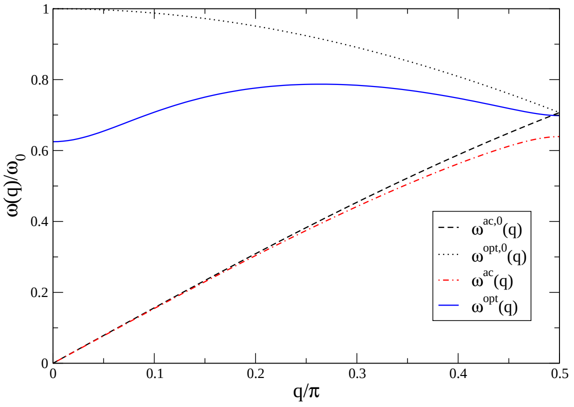


FIG. 1. Dispersion of acoustic phonons $\omega^{\mathrm{ac}}(q)$ and of optical phonons $\omega^{\mathrm{opt}}(q)$ in the Peierls chain as a function of momentum $q$ for $\delta_0 = 0.130$. For comparison we also show the bare dispersions $\omega^{\mathrm{ac},0}(q)$ and $\omega^{\mathrm{opt},0}(q)$ for a spring-constant model without the contributions of the $\pi$ electrons.

### 4. Phonon frequencies for limiting cases

In general, the integrals for $D_{mn}(q)$ must be done numerically. We obtain more compact results for some limiting cases.

*a. Limit of vanishing electron-phonon coupling.* For $\alpha_x = 0$ we have $D_{mn}(q) = 0$ and we find

$$\begin{aligned} \omega^{\mathrm{ac},0}(q) &= \omega_0 |\sin(q/2)| \, , \\ \omega^{\mathrm{opt},0}(q) &= \omega_0 |\cos(q/2)| \, , \\ \omega_0 &= \sqrt{\frac{4K_x}{M}} \end{aligned} \tag{46}$$

for $-\pi/2 \leq q \leq \pi/2$, as expected for a linear chain of atoms. Note that the optical branch in the reduced Brillouin zone complements the acoustic branch when unfolded into the full Brillouin zone, $-\pi < q \leq \pi$. The bare phonons dispersions are shown in Fig. 1 as dashed and dotted lines.

The frequency of the bare optical phonon is given by $\omega_0$. For $M = 12u$ ($1u = 1.66054 \cdot 10^{-27}\,\mathrm{kg}$) and $K_x = 21\,\mathrm{eV/Å}$ we have $\omega_0 = 2.60 \cdot 10^{14}/\mathrm{s} = 1.38 \cdot 10^3\,\mathrm{cm}^{-1}$. This is in the range of optical phonon frequencies measured in trans-polyacetylene.[8]

*b. Renormalized sound velocity.* For $q \to 0$, we have $D_{22}(q \to 0) = D_{22} + Bq^2$, $D_{11}(q \to 0) = D_{11}q^2$, and $|D_{12}(q \to 0)| = |D_{12}|q$ with

$$\begin{aligned} \frac{2D_{11}}{K_x} &= -\frac{8\alpha_x^2}{(K_x/2)} \int_{-\pi/2}^{\pi/2} \frac{\mathrm{d}k}{2\pi} \frac{[2t_0\delta_0 \sin(k)\cos(k)]^2}{2[E(k)]^3} \\ &= -\frac{4\alpha_x^2 \delta_0^2}{K_x t_0} \int_{-\pi/2}^{\pi/2} \frac{\mathrm{d}k}{2\pi} \frac{[\sin(k)\cos(k)]^2}{(\cos^2(k) + \delta_0^2 \sin^2(k))^{3/2}} \\ &= \delta_0^2(-1 + [R(\delta_0)]^2) \, , \end{aligned} \tag{47}$$

$$\begin{aligned} \frac{|D_{12}|}{K_x} &= \frac{8\alpha_x^2}{K_x} \int_{-\pi/2}^{\pi/2} \frac{\mathrm{d}k}{2\pi} \frac{2\sin(k)\cos(k)[4\delta_0 t_0^2 \cos(k)\sin(k)]}{2[E(k)]^3} \\ &= \frac{4\alpha_x^2 \delta_0}{K_x t_0} \int_{-\pi/2}^{\pi/2} \frac{\mathrm{d}k}{2\pi} \frac{[\sin(k)\cos(k)]^2}{(\cos^2(k) + \delta_0^2 \sin^2(k))^{3/2}} \\ &= \frac{2|D_{11}|}{K_x \delta_0} = \delta_0 | -1 + [R(\delta_0)]^2| \, , \end{aligned} \tag{48}$$

$$\begin{aligned} \frac{D_{22}}{2K_x} &= -\frac{8\alpha_x^2}{2K_x} \int_{-\pi/2}^{\pi/2} \frac{\mathrm{d}k}{2\pi} \frac{[2t_0 \cos(k) 2\sin(k)]^2}{2[E(k)]^3} \\ &= -\frac{4\alpha_x^2}{K_x t_0} \int_{-\pi/2}^{\pi/2} \frac{\mathrm{d}k}{2\pi} \frac{[\sin(k)\cos(k)]^2}{(\cos^2(k) + \delta_0^2 \sin^2(k))^{3/2}} \\ &= -1 + [R(\delta_0)]^2 \, , \end{aligned} \tag{49}$$

where, using eq. (20), $R(\delta_0)$ is derived from

$$[R(\delta_0)]^2 = 1 - \frac{\displaystyle\int_{-\pi/2}^{\pi/2} \frac{\mathrm{d}k}{2\pi} \frac{[\sin(k)\cos(k)]^2}{(\cos^2(k) + \delta_0^2 \sin^2(k))^{3/2}}}{\displaystyle\int_{-\pi/2}^{\pi/2} \frac{\mathrm{d}k}{2\pi} \frac{\sin^2(k)}{\sqrt{\cos^2(k) + \delta_0^2 \sin^2(k)}}} \, . \tag{50}$$

As expected, we find a linear dispersion relation for the acoustic phonon

$$\omega^{\mathrm{ac}}(q \to 0) = c_s q \tag{51}$$

with the sound velocity from eq. (45),

$$\begin{aligned} \left(\frac{c_s}{c_{s,0}}\right)^2 &= \frac{(1 + 2D_{11}/K_x)(1 + D_{22}/(2K_x)) - |D_{12}/K_x|^2}{1 + D_{22}/(2K_x)} \\ &= 1 + \delta_0^2 - \left(\frac{\delta_0}{R(\delta_0)}\right)^2 \, . \end{aligned} \tag{52}$$

For $\delta_0 = 0.130$ and thus $R(\delta_0) = 0.625$ we find $c_s/c_s^0 = 0.987$, i.e., the correction is negligibly small. This is also seen in Fig. 1 which shows that the acoustic branch is not strongly influenced by the itinerant degrees of freedom in the whole Brillouin zone, apart from the fact that the slope of $\omega^{\mathrm{ac}}(q)$ vanishes at the Brillouin zone boundary, as it must for a standing wave.

*c. Optical phonon frequency.* For $q = 0$ we have $D_{11}(0) = D_{12}(0) = D_{21}(0) = 0$ and $D_{22}(0) = D_{22}$. We thus find the two solutions $\omega^{\mathrm{ac}}(0) = 0$, as expected for the acoustic branch, and

$$\omega^{\mathrm{opt}}(0) = \omega_0 R(\delta_0) \, . \tag{53}$$

For $\delta_0 = 0.130$ and thus $R(\delta_0) = 0.625$, the optical phonon is renormalized by more than 30%. This softening of the optical phonon as a consequence of the electrons' itineracy is known as Kohn anomaly.[9] As seen from Fig. 1, the Kohn anomaly extends over the whole Brillouin zone, i.e., the optical phonon dispersion $\omega^{\mathrm{opt}}(q)$ lies below the bare optical phonon dispersion $\omega^{\mathrm{opt},0}(q)$ for all $q$. The renormalization at the Brillouin zone boundary $q = \pi/2$ is very small, apart from the fact that $\omega^{\mathrm{opt}}(q)$ has a zero slope as it must for a standing wave.

### 5. Optical phonon frequency from the ground-state energy

The frequency of the optical phonon can be calculated directly from the diagonalization of the Hamiltonian in the presence of the distortion. We can derive the effective spring constant from the general expression for the energy as a function of the distortion, $e_0(u)$ in eq. (19),

$$K_{\mathrm{eff}} = \left.\frac{\partial^2 e_0(u)}{\partial u^2}\right|_{u=u_0} \, . \tag{54}$$

Indeed, we find

$$\begin{aligned} \frac{K_{\mathrm{eff}}}{K_x} &= 1 - 2\int_{-\pi/2}^{\pi_2} \frac{\mathrm{d}k}{2\pi} \frac{4\alpha_x^2 4t_0^2 \sin^2(k)\cos^2(k)}{K_x[\epsilon(k)^2 + \Delta(k)^2]^{3/2}} \\ &= 1 - \frac{4\alpha_x^2}{K_x t_0} \int_{-\pi/2}^{\pi_2} \frac{\mathrm{d}k}{2\pi} \frac{\sin^2(k)\cos^2(k)}{[\cos^2(k) + \delta_0^2 \sin^2(k)]^{3/2}} \\ &= 1 + [-1 + R(\delta_0)^2] = [R(\delta_0)]^2 \, . \end{aligned} \tag{55}$$

Therefore, we recover the result for the optical phonon at $q = 0$ in eq. (53), $\omega^{\mathrm{opt}} = \omega_0\sqrt{K_{\mathrm{eff}}/K_x} = \omega_0 R(\delta_0)$.

## II. HELLMANN-FEYNMAN THEOREM

In this section we derive the Hellmann-Feynman theorem to first and second order.

### A. First-order theorem

Let $\vec{\lambda}$ be a set of variables. Then, the Hamiltonian $\hat{H}(\vec{\lambda})$ and its eigenstate $|\psi(\lambda)\rangle$ with energy $E(\vec{\lambda})$ obey the Schrödinger equation

$$\hat{H}(\vec{\lambda})|\psi(\vec{\lambda})\rangle = E(\vec{\lambda})|\psi(\vec{\lambda})\rangle \; . \tag{56}$$

Likewise we may write

$$E(\vec{\lambda}) = \frac{\langle\psi(\vec{\lambda})|\hat{H}(\vec{\lambda})|\psi(\vec{\lambda})\rangle}{\langle\psi(\vec{\lambda})|\psi(\vec{\lambda})\rangle} \; . \tag{57}$$

In the following, we suppress the dependence of all quantities on $\vec{\lambda}$ and denote the partial derivatives with an index, e.g.,

$$E_i = \frac{\partial E(\vec{\lambda})}{\partial\lambda_i} \quad , \quad |\psi_i\rangle = \frac{\partial|\psi(\vec{\lambda})\rangle}{\partial\lambda_i} \; . \tag{58}$$

Then, the derivative of the energy with respect to the variable $\lambda_i$ can be written as

$$\begin{aligned} E_i = {} & \frac{\langle\psi_i|\hat{H}|\psi\rangle}{\langle\psi|\psi\rangle} + \frac{\langle\psi|\hat{H}_i|\psi\rangle}{\langle\psi|\psi\rangle} + \frac{\langle\psi|\hat{H}|\psi_i\rangle}{\langle\psi|\psi\rangle} \\ & - \frac{\langle\psi|\hat{H}|\psi\rangle}{\langle\psi|\psi\rangle^2}\left(\langle\psi_i|\psi\rangle + \langle\psi|\psi_i\rangle\right) \; . \end{aligned} \tag{59}$$

When we use the Schrödinger equation (56),

$$\langle\psi_i|\hat{H}|\psi\rangle = E\langle\psi_i|\psi\rangle = \frac{\langle\psi|\hat{H}|\psi\rangle}{\langle\psi|\psi\rangle}\langle\psi_i|\psi\rangle \; , \tag{60}$$

we find that the first and the third term in eq. (59) are canceled by the fourth and the fifth term. Thus,

$$E_i \equiv \frac{\partial E(\vec{\lambda})}{\partial\lambda_i} = \frac{\langle\psi(\vec{\lambda})|\partial\hat{H}(\vec{\lambda})/\partial\lambda_i|\psi(\vec{\lambda})\rangle}{\langle\psi(\vec{\lambda})|\psi(\vec{\lambda})\rangle} \equiv \frac{\langle\psi|\hat{H}_i|\psi\rangle}{\langle\psi|\psi\rangle} \; . \tag{61}$$

This is the Hellmann-Feynman theorem to first order.[10–12]

### B. Second-order theorem

We go one step further and study the second-order derivatives, starting from the Hellmann-Feynman theorem (61)

$$\begin{aligned} E_{i,j} = {} & \frac{\langle\psi_j|\hat{H}_i|\psi\rangle}{\langle\psi|\psi\rangle} + \frac{\langle\psi|\hat{H}_{i,j}|\psi\rangle}{\langle\psi|\psi\rangle} + \frac{\langle\psi|\hat{H}_i|\psi_j\rangle}{\langle\psi|\psi\rangle} \\ & - \frac{\langle\psi|\hat{H}_i|\psi\rangle}{\langle\psi|\psi\rangle^2}\left(\langle\psi_j|\psi\rangle + \langle\psi|\psi_j\rangle\right) \; . \end{aligned} \tag{62}$$

We specialize to the case where we seek the Taylor expansion of the ground state where

$$\left.\frac{\partial E(\vec{\lambda})}{\partial\lambda_i}\right|_{\vec{\lambda}=\vec{\lambda}_0} \equiv E_i(\vec{\lambda}_0) = 0 \; . \tag{63}$$

Then, the last two terms in eq. (62) vanish and we are left with

$$E_{i,j}(\vec{\lambda}_0) = \frac{\langle\psi_j|\hat{H}_i|\psi\rangle}{\langle\psi|\psi\rangle} + \frac{\langle\psi|\hat{H}_{i,j}|\psi\rangle}{\langle\psi|\psi\rangle} + \frac{\langle\psi|\hat{H}_i|\psi_j\rangle}{\langle\psi|\psi\rangle} \; , \tag{64}$$

and all objects are evaluated at $\vec{\lambda} = \vec{\lambda}_0$. The derivative of the Schrödinger equation (56) leads to

$$\hat{H}_i(\vec{\lambda}_0)|\psi(\vec{\lambda}_0)\rangle + \hat{H}(\vec{\lambda}_0)|\psi_i(\vec{\lambda}_0)\rangle = E(\vec{\lambda}_0)|\psi_i(\vec{\lambda}_0)\rangle \tag{65}$$

when evaluated at $\vec{\lambda} = \vec{\lambda}_0$ where $E_i(\vec{\lambda}_0) = 0$. Therefore, $|\psi_i\rangle$ is nothing but the correction vector

$$|\psi_i(\vec{\lambda}_0)\rangle = -\left(\hat{H}(\vec{\lambda}_0) - E(\vec{\lambda}_0)\right)^{-1}\hat{H}_i(\vec{\lambda}_0)|\psi(\vec{\lambda}_0)\rangle \; . \tag{66}$$

The explicit calculation of the correction vector can be avoided, see below. Inserting (66) into (64), the second-order Taylor coefficients of the ground-state energy expanded around the equilibrium values read

$$\begin{aligned} E_{i,j}(\vec{\lambda}_0) = {} & \left\langle \frac{\partial^2\hat{H}(\vec{\lambda})}{\partial\lambda_i\partial\lambda_j} \right\rangle \\ & - \left\langle \frac{\partial\hat{H}(\vec{\lambda})}{\partial\lambda_i}\left(\frac{1}{\hat{H}(\vec{\lambda}) - E(\vec{\lambda})}\right)\frac{\partial\hat{H}(\vec{\lambda})}{\partial\lambda_j} \right\rangle \\ & - \left\langle \frac{\partial\hat{H}(\vec{\lambda})}{\partial\lambda_j}\left(\frac{1}{\hat{H}(\vec{\lambda}) - E(\vec{\lambda})}\right)\frac{\partial\hat{H}(\vec{\lambda})}{\partial\lambda_i} \right\rangle \; , \end{aligned} \tag{67}$$

where, for an operator $\hat{A}$,

$$\langle\hat{A}\rangle \equiv \frac{\langle\psi(\vec{\lambda}_0)|\hat{A}(\vec{\lambda}_0)|\psi(\vec{\lambda}_0)\rangle}{\langle\psi(\vec{\lambda}_0)|\psi(\vec{\lambda}_0)\rangle} \; . \tag{68}$$

Equation (67) constitutes the second-order Hellmann-Feynman theorem.

The static correlation functions in the second-order Hellmann-Feynman theorem (67) can be calculated in various ways. Following Shirakawa and Jeckelmann[13] (see also Ref. [14]) we define the real functional for the Hermitian operator $\hat{A}$

$$W_\varphi(\hat{A})\langle\psi|\psi\rangle = \langle\varphi|\hat{H} - E_0|\varphi\rangle - \langle\psi|\hat{A}|\varphi\rangle - \langle\varphi|\hat{A}|\psi\rangle \; . \tag{69}$$

Note that $\hat{H} \equiv \hat{H}(\vec{\lambda}_0)$, $E_0 \equiv E(\vec{\lambda}_0)$ and $|\psi\rangle \equiv |\psi(\vec{\lambda}_0)\rangle$. Optimizing this functional with respect to $|\varphi\rangle$, and $\langle\varphi|$ gives

$$W^{\rm opt}(\hat{A}) = W_{\varphi^{\rm opt}}(\hat{A}) = -\left\langle \hat{A}\left(\frac{1}{\hat{H} - E_0}\right)\hat{A} \right\rangle \; . \tag{70}$$

With this result we can cast eq. (67) into the form

$$\begin{aligned} E_{i,j}(\vec{\lambda}_0) = &\left\langle \frac{\partial^2 \hat{H}(\vec{\lambda})}{\partial\lambda_i \partial\lambda_j} \right\rangle \\ &+W^{\rm opt}\left(H_i(\vec{\lambda}_0)+H_j(\vec{\lambda}_0)\right) \\ &-W^{\rm opt}\left(H_i(\vec{\lambda}_0)\right)-W^{\rm opt}\left(H_j(\vec{\lambda}_0)\right) \, . \end{aligned} \quad (71)$$

This form of the Hellmann-Feynman theorem can be used for a calculation of the dynamical matrix that avoids the use of finite distortions and the corresponding extrapolations.

## III. DERIVATION OF ENERGY GRADIENTS

For the calculation of energy gradients we need the derivatives of the total energy with respect to $x_n$ and $y_n$. For our numerical analysis, we have $L_C = 2L+2$ sites, and we fix the positions of the first and last atoms ($n = 0, 2L+1$).

### A. Gradient with respect to $x_n$

For $n = 1, \ldots, 2L$, the derivatives with respect to $x_n$ read

$$\begin{aligned} \frac{\partial E_{\rm el}}{\partial x_n} = &\sum_\sigma \frac{\alpha}{t_0}\left[\frac{t_{n-1}(x_{n-1}-x_n)}{d_{n-1}}P_{n-1,\sigma} \right. \\ &\left. - \frac{t_n(x_{n+1}-x_n)}{d_n}P_{n,\sigma}\right] \quad (72) \\ &-\frac{V\beta}{\epsilon_d (\text{Å})^2}\sum_{j=0,j\neq n}^{2L+1}\frac{C_{nj}(x_n-x_j)}{\left(1+\beta\left(d_{nj}/\text{Å}\right)^2\right)^{3/2}} \, , \end{aligned}$$

$$\frac{\partial E_{\rm CC}}{\partial x_n} = V'_\sigma(d_{n-1})\frac{x_n-x_{n-1}}{d_{n-1}} - V'_\sigma(d_n)\frac{x_{n+1}-x_n}{d_n} \, , \quad (73)$$

$$\begin{aligned} \frac{1}{C_{\rm b}}\frac{\partial E_{\rm CC\,b}}{\partial x_n} = &(1-\delta_{n,1})(\cos(\vartheta_{n-1})-\cos(\Theta_0))\frac{\partial\tilde{\vartheta}_{n-1}}{\partial x_n} \\ &+(\cos(\vartheta_n)-\cos(\Theta_0))\frac{\partial\tilde{\vartheta}_n}{\partial x_n} \\ &+(1-\delta_{n,2L})(\cos(\vartheta_{n+1})-\cos(\Theta_0))\frac{\partial\tilde{\vartheta}_{n+1}}{\partial x_n} . \end{aligned} \quad (74)$$

Here,

$$V'_\sigma(r) = K_{\sigma,0} + K_{\sigma,1}(r-r_0) \quad (75)$$

is the derivative of the $\sigma$-bond potential, and we introduced the following abbreviations,

$$\begin{aligned} \frac{\partial\tilde{\vartheta}_{n-1}}{\partial x_n} = &-\frac{x_{n-1}-x_{n-2}}{d_{n-1}d_{n-2}} \\ &+\frac{(x_n-x_{n-1})(x_n-x_{n-1})(x_{n-1}-x_{n-2})}{d_{n-1}^3 d_{n-2}} \\ &+\frac{(x_n-x_{n-1})(y_n-y_{n-1})(y_{n-1}-y_{n-2})}{d_{n-1}^3 d_{n-2}} \, , \end{aligned} \quad (76)$$

$$\begin{aligned} \frac{\partial\tilde{\vartheta}_n}{\partial x_n} = &\frac{(x_n-x_{n-1})(x_{n+1}-x_n)(x_n-x_{n-1})}{d_{n-1}^3 d_n} \\ &+\frac{(x_n-x_{n-1})(y_{n+1}-y_n)(y_n-y_{n-1})}{d_{n-1}^3 d_n} \\ &+\frac{2x_n-x_{n-1}-x_{n+1}}{d_n d_{n-1}} \\ &-\frac{(x_{n+1}-x_n)(x_{n+1}-x_n)(x_n-x_{n-1})}{d_n^3 d_{n-1}} \\ &-\frac{(x_{n+1}-x_n)(y_{n+1}-y_n)(y_n-y_{n-1})}{d_n^3 d_{n-1}} \, , \end{aligned} \quad (77)$$

$$\begin{aligned} \frac{\partial\tilde{\vartheta}_{n+1}}{\partial x_n} = &\frac{x_{n+2}-x_{n+1}}{d_n d_{n+1}} \\ &-\frac{(x_{n+1}-x_n)(x_{n+1}-x_n)(x_{n+2}-x_{n+1})}{d_n^3 d_{n+1}} \\ &-\frac{(x_{n+1}-x_n)(y_{n+1}-y_n)(y_{n+2}-y_{n+1})}{d_n^3 d_{n+1}} \, . \end{aligned} \quad (78)$$

### B. Gradient with respect to $y_n$ ($y_3 = 0$)

For the derivatives with respect to $y_n$ we simply replace $x_n \leftrightarrow y_n$. For completeness, we compile the resulting expressions.

$$\begin{aligned} \frac{\partial E_{\rm el}}{\partial y_n} = &\sum_\sigma \frac{\alpha}{t_0}\left[\frac{t_{n-1}(y_{n-1}-y_n)}{d_{n-1}}P_{n-1,\sigma} \right. \\ &\left. - \frac{t_n(y_{n+1}-y_n)}{d_n}P_{n,\sigma}\right] \quad (79) \\ &-\frac{V\beta}{\epsilon_d (\text{Å})^2}\sum_{j=0,j\neq n}^{2L+1}\frac{C_{nj}(y_n-y_j)}{\left(1+\beta\left(d_{nj}/\text{Å}\right)^2\right)^{3/2}} \, , \end{aligned}$$

$$\frac{\partial E_{\rm CC}}{\partial y_n} = V'_\sigma(d_{n-1})\frac{y_n-y_{n-1}}{d_{n-1}} - V'_\sigma(d_n)\frac{y_{n+1}-y_n}{d_n} \, , \quad (80)$$

$$\frac{1}{C_{\rm b}}\frac{\partial E_{\rm CC\,b}}{\partial y_n} = (1-\delta_{n,1})(\cos(\vartheta_{n-1})-\cos(\Theta_0))\frac{\partial\tilde{\vartheta}_{n-1}}{\partial y_n} +(\cos(\vartheta_n)-\cos(\Theta_0))\frac{\partial\tilde{\vartheta}_n}{\partial y_n} +(1-\delta_{n,2L})(\cos(\vartheta_{n+1})-\cos(\Theta_0))\frac{\partial\tilde{\vartheta}_{n+1}}{\partial y_n}. \quad (81)$$

We introduced the following abbreviations,

$$\frac{\partial\tilde{\vartheta}_{n-1}}{\partial y_n} = -\frac{y_{n-1}-y_{n-2}}{d_{n-1}d_{n-2}} +\frac{(y_n-y_{n-1})(y_n-y_{n-1})(y_{n-1}-y_{n-2})}{d_{n-1}^3 d_{n-2}} +\frac{(y_n-y_{n-1})(x_n-x_{n-1})(x_{n-1}-x_{n-2})}{d_{n-1}^3 d_{n-2}}, \quad (82)$$

$$\frac{\partial\tilde{\vartheta}_n}{\partial y_n} = \frac{(y_n-y_{n-1})(y_{n+1}-y_n)(y_n-y_{n-1})}{d_{n-1}^3 d_n} +\frac{(y_n-y_{n-1})(x_{n+1}-x_n)(x_n-x_{n-1})}{d_{n-1}^3 d_n} +\frac{2y_n-y_{n-1}-y_{n+1}}{d_n d_{n-1}} -\frac{(y_{n+1}-y_n)(y_{n+1}-y_n)(y_n-y_{n-1})}{d_n^3 d_{n-1}} -\frac{(y_{n+1}-y_n)(x_{n+1}-x_n)(x_n-x_{n-1})}{d_n^3 d_{n-1}}, \quad (83)$$

$$\frac{\partial\tilde{\vartheta}_{n+1}}{\partial y_n} = \frac{y_{n+2}-y_{n+1}}{d_n d_{n+1}} -\frac{(y_{n+1}-y_n)(y_{n+1}-y_n)(y_{n+2}-y_{n+1})}{d_n^3 d_{n+1}} -\frac{(y_{n+1}-y_n)(x_{n+1}-x_n)(x_{n+2}-x_{n+1})}{d_n^3 d_{n+1}}. \quad (84)$$

---

* florian.gebhard@physik.uni-marburg.de
† legeza.ors@wigner.mta.hu

[1] A. J. Heeger, S. Kivelson, J. R. Schrieffer and W.-P. Su, *Rev. Mod. Phys.*, 1988, **60**, 781–850.
[2] Note that in Ref. [1], $u^{\rm SSH} = 2u$.
[3] F. Gebhard, K. Bott, M. Scheidler, P. Thomas and S. W. Koch, *Philosophical Magazine Part B*, 1997, **75**, 1–12.
[4] *Mathematica, Version 9.0*, Wolfram Research, Inc., Champaign, 2012.
[5] H. J. Schulz, *Phys. Rev. B*, 1978, **18**, 5756–5767.
[6] E. J. Mele and M. J. Rice, *Solid State Communications*, 1980, **34**, 339–342.
[7] K. A. Chao and Y. Wang, *Physica Scripta*, 1986, **34**, 177.
[8] H. Kuzmany, *physica status solidi (b)*, 1980, **97**, 521–531.
[9] W. Kohn, *Phys. Rev. Lett.*, 1959, **2**, 393–394.
[10] H. Hellmann, *Einführung in die Quantenchemie*, Deuticke, Leipzig und Wien, 1937.
[11] H. Hellmann, *Einführung in die Quantenchemie*, Springer, Berlin, 2015.
[12] R. P. Feynman, *Phys. Rev.*, 1939, **56**, 340–343.
[13] T. Shirakawa and E. Jeckelmann, *Phys. Rev. B*, 2009, **79**, 195121.
[14] P. Schmitteckert and R. Werner, *Phys. Rev. B*, 2004, **69**, 195115.
